# Supplementary material for: SCORCH. III. Analytical Models of Reionization with Varying Clumping Factors
Source: arXiv:2004.07854 source file (2021-01-26)
Supplement: Supplementary file 1 [file appendix.tex]

\appendix
